# Supplementary material for: Ultrafast Hot-Carrier Dynamics in Ultrathin Monocrystalline Gold
Source: arXiv:2311.08131 source file (2023-11-14)
Supplement: Supplementary file 1 [file appendix1.tex]

\section{SI1-Transient Reflectivity Simulations} \label{sec:appendix_SI1}

The optical properties of metal can be described as two coupled thermal systems made up of the electron and the phonon baths when nonequilibrium electron heating is being considered\cite{PhysRevLett.58.1680,PhysRevB.50.15337}. A phenomenological description of the evolution of the electron gas can be obtained 
considering the nonthermalized electron distribution, created by the absorbed pump pulse, which acts as a heat reservoir and decays by exchanging energy through electron-electron scattering with the colder electrons until the electron system reaches thermal equilibrium. Electron-phonon scattering then equilibrates the temperatures of the electron and lattice subsystems. By taking into account the energy content of the electron gas, the pump-induced evolution of the coupled electron-phonon system can be described by three coupled differential equations as \cite{PhysRevB.50.15337}
\begin{equation}\label{3ttm1}
\frac{\partial N(t)}{\partial t}=-\overline{\gamma_{e}}N(t)-bN(t)+P_{abs}(t)
\end{equation}
\begin{equation}\label{3ttm2}
C_e\frac{\partial T_e(t)}{\partial t}=-G(T_e(t)-T_l(t))+aN(t)
\end{equation}
\begin{equation}\label{3ttm3}
C_l\frac{\partial T_l(t)}{\partial t}=G(T_e(t)-T_l(t))+bN(t)
\end{equation}
where $C_e$ and $C_l$ are the electron and lattice heat capacities, $T_e$ and $T_l$ are the electron and lattice temperatures, respectively, $G$ is the electron-phonon coupling constant, $N$ is the variable describing the energy density stored in the nonthermalized part of the distribution, $\overline{\gamma_{e}}$ is the average scattering rate of the nonthermalized electrons, which is described by an average of $\tau^{-1}_{ee}(\varepsilon)=\gamma_{ee}(\varepsilon)=(D_e/\hbar)(\varepsilon)^2$ \cite{PhysRevLett.118.087401,PhysRevB.94.075120}, and $b$ is the electron-phonon coupling rate. $P_{abs}$ is the absorbed pump-pulse power in the unit volume of the metal, which depends on a pump fluence F as
\begin{equation}\label{pabs}
P_{abs}(t)= \sqrt{\frac{2}{\pi}}\frac{Abs(\lambda)F}{L\tau_p}exp(-2t^2/\tau_p^2)
\end{equation}
where $Abs(\lambda)$ is the absorption at the pump wavelength, $L$ is the thickness of the metal, $\tau_p$ is the half width of the pump pulse at $1/e^2$ power.
The corresponding pump-induced change in the thermalized and nonthermalized electron occupancy is given by \cite{Zavelani-Rossi2015,PhysRevB.86.155139,PhysRevB.89.125122}
\begin{equation} \label{deltathermalized}
    \Delta f_T(\varepsilon,t)=f_0(\varepsilon,T_e(t))-f_0(\varepsilon,T_0)
\end{equation}
\begin{equation} \label{deltanonthermalized}
    \Delta f_{NT}(\varepsilon,t)= C*\Delta_{NT}(\varepsilon)\int_{-\infty}^{t}P_a(t')e^{-(t-t')/\tau(\varepsilon)}dt'
\end{equation}
where $f_0$ is the Fermi-Dirac distribution and $\Delta_{NT}(\epsilon)=f_0(\varepsilon-\hbar\omega_{pump})*[1-f_0(\varepsilon)]-f_0(\varepsilon)[1-f_0(\varepsilon+\hbar\omega_{pump})]$. The normalization constant can be found from the energy conservation law as \cite{PhysRevB.86.155139}
\begin{equation}
    C=\int\Delta_{NT}(E)DOS(E)EdE
\end{equation}
where $DOS(E)$ is the energy density states of Au. 
The pump-induced change in the occupancy of thermalized and nonthermalized electron states causes the modulation of the interband transition in Au as $\Delta\epsilon_{T}(\hbar\omega,t)$ and $\Delta\epsilon_{NT}(\hbar\omega,t)$, respectively. The imaginary part of these quantities can be computed under the constant matrix element approximation in the parabolic band approximation as follows \cite{Zavelani-Rossi2015,PhysRevB.89.125122,JDOS_1,JDOS_2,PhysRevB.85.235403} :
\begin{equation}
    \Im[\Delta\epsilon_{T(NT)}(\hbar\omega,t)]=\frac{A_XJ_X_{T(NT)}(\hbar\omega,t)+A_{L_4^+}J_{L_4^+}_{T(NT)}(\hbar\omega,t)+A_L_{5+6}^+J_L_{5+6}^+_{T(NT)}(\hbar\omega,t)}{\hbar\omega^2}
\end{equation}
where 
\begin{equation}
    J_i_{T(NT)}(\hbar\omega,t)=\int_{E_{min}}^{E_{max}}D_i(E,\hbar\omega)\Delta f_{T(NT)}(E,t)dE,
\end{equation}
are the joint density of states (JDOS), $D_i(E,\hbar\omega)$ are the energy distribution of the joint density of states (EDJDOS), and $A_i$ are the squares of the momentum operator matrix element describing the transition strength for the corresponding transitions with $i=X,L_4^+,L_{5+6}^+$. The reduced masses of the electrons in bands, energy separations between the bands at high symmetry points, and the integration limits are taken from ref \cite{PhysRevB.85.235403}. The corresponding pump-induced transient change in the real part of $\Delta\epsilon_{T(NT)}(\hbar\omega,t)$ is calculated using the Kramers-Kronig analysis.

% \begin{figure*}[h]
% \centering
% \begin{subfigure}{.65\textwidth} 
% \hspace{-5.5cm}
%   \centering
%   \includegraphics[width=0.8\linewidth]{images/DRvsF.eps}
%   \caption{\hspace{5.5cm} }
%   \label{figS1_1_a}
% \end{subfigure}%
% \begin{subfigure}{.65\textwidth}
% \hspace{-6.5cm}
%   \centering
%   \includegraphics[width=0.8\linewidth]{images/Delta_epsilon_T_NT_025-1-2-3-4-5.eps}
%   \caption{\hspace{5.5cm} }
%   \label{figS1_1_b}
% \end{subfigure}
% \begin{subfigure}{.65\textwidth}
% \hspace{}
%   \centering
%   \includegraphics[width=0.8\linewidth]{images/JDOSX.png}
%   \caption{}
%   \label{figS1_1_c}
% \end{subfigure}

\caption{ \justifying { Simulated (a) $\Delta R/R$ and (b) $\Delta\epsilon_{T}(t)$ and $\Delta\epsilon_{NT}(t)$} at different laser fluences, indicated in the panels. (c) JDOS of Au at X point at different electron temperatures $T_e$.}
\label{figS1_1}
\end{figure*}

The induced changes in the intraband permittivity are calculated through the Drude-Sommerfeld model. The intraband permittivity is described as  
\begin{equation}\label{epsilon}
\epsilon_{intraband}=\epsilon_{inf}-\frac{\omega_p^2}{\omega(\omega+i\Gamma(\hbar\omega,T_e,T_l))}
\end{equation}
$\omega_p=9.02 eV$ is the plasma frequency of Au and $\epsilon_{inf}=3$ was set to fit the Johnson-Christy data for Au permittivity 
\cite{PhysRevB.6.4370,Neira2015}. Pump-induced modulation of the Drude damping parameter, $\Gamma(T_e,T_l)$, is defined as 
\begin{equation}
\Gamma(T_e,T_l)=\Gamma_{e-e}(\hbar\omega,T_e)+\Gamma_{e-ph}(T_l)
\end{equation}
where 
\begin{equation}\label{tauee_2}
\Gamma_{e-e}(\hbar\omega,T_e)=\frac{1}{12}\pi^3\beta\Delta(1/\hbar E_F)[(k_BT_e)^2+\hbar\omega^2]
\end{equation}
and the Holstein's expression \cite{ephh}
\begin{equation}\label{tph}
\Gamma_{e-ph}(T_l)=\frac{1}{\tau_0}\bigg[\frac{2}{5}   +  4\bigg(\frac{T_l}{\Theta}\bigg)^5\int_{0}^{\Theta/T_l} \frac{z^4}{e^z-1}dz\bigg].
\end{equation}
where $E_F$= 5.55 eV is the Fermi energy of Au, $\beta$ is a constant giving an average electron scattering probability over the Fermi surface, which is approximately 0.55 for noble metals, $\Delta$ is the fractional Umpklapp scattering, approximately 0.75 \cite{tau}, $\Theta$ is the Debye temperature, which is 170 K for Au, and a $1/\tau_0$ is a constant, which is 0.007 eV for Au by fitting the Au bulk permittivity at a frequency below 2.5 eV which is a gold interband transition onset \cite{e-ph2}. Then, the computed $\Delta\epsilon(\hbar\omega,t)$ is fed into the simulations of $\Delta R(t)/R$ via the transfer matrix method.
