# Supplementary material for: Ultrafast Hot-Carrier Dynamics in Ultrathin Monocrystalline Gold
Source: arXiv:2311.08131 source file (2023-11-14)
Supplement: Supplementary file 2 [file appendix2.tex]

\section{SI2-Hot electron transfer efficiency simulation} \label{sec:appendix_SI2}

The probability that an electron is excited to particular energy, E = E$_F$ + $\varepsilon$, is given by the product of the electron density of states, g($\varepsilon$), at the initial and final electron energies, normalized by the same product integrated over all possible initial and final electron energy combinations:
\begin{equation}
    P_{\varepsilon}(\varepsilon)= \frac{g(\varepsilon+E_F) g(\varepsilon+E_F-h\nu) }{ \bigintss_{E_F}^{E_F+h\nu} g(E^{'}) g(E^{'}-h\nu) dE^{'}}
\end{equation}
where $h\nu$ is the pump photon energy. We assume that the parabolic band approximation applicable for the intraband transitions, so that $g(\varepsilon)\propto \sqrt{\varepsilon}$. 
We assume that electron-phonon scattering causes a minimal loss of energy of for the hot electron, and the main energy loss takes place through e-e scattering. The probability that the hot electron will reach the interface in the case of electron-electron scattering is determined by the mean free path, $\lambda_e$:
\begin{equation}
P_r(t,\varepsilon)=\bigintsss_{0}^{t} \bigintsss_{-\pi/2}^{\pi/2} \frac{1}{t} \frac{1}{2\pi} e^{\frac{-z}{cos\theta \lambda_e(\varepsilon)}}  e^{\frac{-z}{\lambda_p}} dzd\theta
\end{equation}
where t is the thickness of Au, $\theta$ is the angle between the normal to the interface and the direction of electron propagation, $\lambda_p$ is the penetration depth of the incoming photon, and $z$ is the normal distance from the interface. The factors of the $1/t$ and $1/2\pi$ come from assuming an equal number of electrons in all $dz$ and isotropic momentum distribution, respectively. 
The total probability $P(h\nu)$ for an excited electron generated by an incident photon of energy $h\nu$ to be injected into a semiconductor can be written as
\begin{equation}
    P(h\nu)=\bigintsss_{\phi_b}^{h\nu} P_\varepsilon(\varepsilon)P_r(t,\varepsilon) d\varepsilon
\end{equation}
where $\phi_b$ is a barrier height. MThus, the fraction of the absorbed energy injected into the semiconductor by the transferred hot electrons, P$_i$, is \cite{Ratchford2017}: 
\begin{equation} \label{pi_expre}
    P_i(h\nu)=\bigintsss_{\phi_b}^{h\nu} \frac{\varepsilon}{h\nu} P_\varepsilon(\varepsilon)P_r(t,\varepsilon) d\varepsilon
\end{equation}

The efficiency of hot electron transfer from the nanoparticles into a semiconductor can be calculated using ref \cite{Ratchford2017}. 

The simulations show that Au nanoparticles embedded in the semiconductor have a higher probability of injection of hot electrons, therefore, higher amount of absorbed energy is transferred compared to the Au slab (Fig. \ref{eff_cases}). It is obvious that as the thickness (diameter) of Au slab (nanoparticle) decreases, P, P$_i$, and P$_r$ increase.
