# Supplementary material for: Ultrafast Hot-Carrier Dynamics in Ultrathin Monocrystalline Gold
Source: arXiv:2311.08131 source file (2023-11-14)
Supplement: Supplementary file 3 [file appendix3.tex]

\section{SI3-Methods}

\subsection{Sample fabrication.}
The high aspect-ratio ultrathin monocrystalline Au MFs with a range of thickness 10--25 nm were fabricated by the procedure 
described in Ref. \cite{doi:10.1021/acs.chemmater.1c03908}. MF has atomically smooth and well-defined $\{111\}$ crystallographic surface and face-centered cubic crystal 
structure (Figs. \ref{optical_image} and \ref{figsi31c}). The RMS roughness of the surface of the flakes is measured to be $\approx$ 250 pm. MF are grown on a 180 $\mu$m thick borosilicate glass substrate. To study the hot electron transfer, the chemically synthesized MFs are 
transferred to the 40 nm thick TiO$_2$ films on a borosilicate glass by the PMMA transfer method 
\cite{https://doi.org/10.1002/smtd.201900049}.  

To compare the effect of crystallinity on hot-carrier properties, 15 nm and 10 nm Au thin-films were fabricated on the same type of substrates by magnetron sputtering. AFM analysis ws used to verify that there are no discontinuities of the 10 nm thick Au thin-film.

\subsection{Optical measurements.}

The transient optical measurements were conducted using a femtosecond laser (Laser Quantum Venteon) and a degenerate pump-probe setup (Fig.\ref{figsi31a}). The laser produced pulses of approximately 8 fs with a repetition rate of 80 MHz, and an average power of around 0.5 W. The spectrum of a such short laser pulse covers a range from 650 to 950 nm (Fig. \ref{figsi31b}). %Since the objective numerical aperture is 0.4 and the incident angle of the pump is 45$^{\circ}$, by parabolic mirrors, none of the pump beams is directly collected by the objective and polluted the measurements. 
The pump and probe beams were cross-polarized in order to prevent coherent interactions during the measurements. The measurement of $\Delta R/R$ was conducted using a lock-in amplifier, which allowed for accurate measurements with a precision of $10^{-6}$ to $10^{-7}$. The pump beam was sent through a mechanical delay stage and chopped at a rate of 1 kHz. The experimental setup included a dispersion control system (Sphere Photonics D-Scan) in order to control the dispersion of the ultashort pulses. To assure consistency, $\Delta R/R$ traces of each sample were measured several times over a few different days.
